# Supplementary material for: Dynamic Textual Prompt For Rehearsal-free Lifelong Person Re-identification
Source: arXiv:2411.06023 source file (2024-11-09)
Supplement: Supplementary file 1 [file 6_supp.tex]

\clearpage
\setcounter{page}{1}

\section{Appendix}
\appendix
The section can be succinctly summarized as follows:

\noindent{1. }

\noindent{2. We give detailed ablation to demonstrate the suporitity of our method in the aspect of alleviating forgetting and enhancing generalziation.}

\noindent{3. We further compare our method with other methods on more training orders and achieve promsing results on disrupted training orders, indicating the superior performance of our method is not yield from any specific training order.}

\section{More visualization results}

\section{Additional experiments}
\begin{table}
  \centering
  \begin{tabular}{c|cc|cc}
    \toprule
     \multirow{2}*{Method} & \multicolumn{2}{c|}{Seen-Avg}& \multicolumn{2}{c}{Uneen-Avg}\\
         &$\bar{S}_{mAP}$ &$\bar{S}_{R1}$ & $\bar{S}_{mAP}$ &$\bar{S}_{R1}$\\
    \hline 
    CRL (WACV21)& $59.3$ & $77.3$ & - & $41.6$\\ 
    GwFRelID (AAAI21) &$53.7$&$71.1$&-&$40.2$\\ 
    PTKP\footnotemark[1](AAAI22)&$67.6$&$81.4$&-&$52.4$\\ 
    ConRFL\footnotemark[1](PR23)&$70.7$&$83.3$ & $49.2$ & $54.1$ \\
    DTP (Ours) &$\textbf{74.0}$ &$\textbf{86.2}$ & $\textbf{68.1}$ & $\textbf{63.0}$\\
    \bottomrule
  \end{tabular}
  \caption{Results for Order-5: We train the model with the order of MA$\rightarrow$DU$\rightarrow$SY$\rightarrow$MS, and test all seen and unseen datasets after the last training stage of MS is completed. Additionally, $*$ demonstrates the data-replay methods.}
  \label{tab:p5ba}
\end{table}
\noindent{\textbf{We can achieve the superior results over more training orders.}} 
Folowing the previous work~\cite{conrfl}, another training order (Order-5) is  MA$\rightarrow$DU$\rightarrow$SY$\rightarrow$MS. The unseen test dataset is CUHK01, CUHK03, grid, sensereid.
% \noindent{\textbf{Extra comparisons with SOTAs.}}
We demonstrate the effectiveness of our DTP method for balanced and imbalanced datasets in Tab.~\ref{tab:p5ba}. Our DTP significantly outperforms all competitors, which leads to $3.3\%$ increase in $\bar{S}_{R1}$ and $2.9\%$ increase in $ \bar{S}_{mAP}$ on seen datasets, and $18.9\%$ increase in $\bar{S}_{R1}$ and $8.9\%$ increase in $\bar{S}_{mAP}$ on unseen datasets.
The results substantiate the efficacy of our method in Order-5, surpassing significantly of ConRFL~\cite{MRN}.
